# Supplementary material for: Measurement of the $\psi(2S)$ to $J/\psi$ cross-section ratio as a function of centrality in PbPb collisions at $\sqrt{s_{\text{NN}}}$ = 5.02 TeV
Source: arXiv:2411.05669 source file (2025-11-13)
Supplement: Supplementary file 1 [file appendix.tex]

% ===============================================================================
% Purpose: appendix to the standard template: standard symbol alises from Ulrik
% Author: Tomasz Skwarnicki
% Created on: 2009-09-24
% ===============================================================================

%{\noindent\normalfont\bfseries\Large Appendices}
%\section*{Appendices}
